# Supplementary material for: Scalable Training of Mixture-of-Experts Models with Megatron Core
Source: arXiv:2603.07685 source file (2026-03-10)
Supplement: Supplementary file 1 [file appendix.tex]

\subsection{Full Example Configuration}
A comprehensive example configuration for Mixtral 8×7B training with recommended optimizations:

\begin{verbatim}
torchrun –nproc_per_node=8 pretrain_gpt.py 
–num-experts 8 
–expert-model-parallel-size 8 
–moe-grouped-gemm 
–moe-permute-fusion 
–moe-router-load-balancing-type aux_loss 
–moe-router-topk 2 
–moe-aux-loss-coeff 1e-2 
–fp8 
–overlap-param-gather 
–overlap-grad-reduce 
–tp-comm-overlap 
–moe-expert-capacity-factor 1.0 
–moe-pad-expert-input-to-capacity 
–tensor-model-parallel-size 1 
–pipeline-model-parallel-size 4 
–num-layers-per-virtual-pipeline-stage 8 
–sequence-parallel 
–use-distributed-optimizer 
–moe-token-dispatcher-type flex 
–moe-enable-deepep 
–recompute-granularity selective 
–recompute-modules moe_act,layernorm 
–moe-use-upcycling
\end{verbatim}
